# Supplementary material for: UWB-ED: Distance Enlargement Attack Detection in Ultra-Wideband
Source: arXiv:1911.11078 source file (2019-11-25)
Supplement: Supplementary file 1 [file appendix.tex]

\section{Appendix}

\todo{Double check the following before submission.}

Whole paper:
\begin{itemize}
\item Use $\delta$ for delay and legitimate distance instead D in paper.
\end{itemize}

Background:
\begin{itemize}

%--regular background
\item Discuss two way ranging in background, and how the ToF is mapped to distance, as well as the sensitivity and precision of common devices and implementations
\item Explain that in ranging, normally taking the highest peak should be sufficient because peaks due to noise should be much lower.

\item Explain how the receiver assembles the signal in the context of PR (phase does not matter, etc), and how the attacker's energy could either add or cancel the signal. Explain also how the very narrow window of UWB gives hope to address this problem because otherwise the adversary could always vanish the pulses completely from the channel

\item In IEEE 802.15.4f, the preamble is a sequence of pulses repeated after a fixed interval of time. The energy and the PRF can be fixed or chosen at random based on the channel condition. The IEEE 802.15.4a use ternary codes, where pulses are modulated using BPSK modulation. However, both codes are predictable and all allow possibility of annihilation. Due to annihilation, no any signal will be received at the receiver, hence packet can go unnoticed. In the non-coherent/Energy-detector (ED) receivers, the decisions are based on aggregated energy at particular positions. Due to annihilation of signal, the energy vanish and attacker get chance to perform enlargement attack.  The annihilation of signal can occur due to channel condition or cancellation  of signal by the attacker. The effect of the channel condition can be mitigated by increasing length of the preamble. This is commonly used techniques, mentioned in standards and off-the-shelf devices allow multiple preamble lengths. However, increasing preamble length does not prevent annihilation due to signal cancellation. 

%--Attack explanation
\item Add in explanation of an attack section: Although the problem may seem to be an authentication problem, it is not since here the adversary is not trying to impersonate the authentic signals, it is rather trying the opposite: trick the receiver into denying that the authentic signals are actually from the receiver.
\item Relying on the first peak. To verify that the committed distance has not been enlarged, the receiver can simply assume the first peak in the preamble is the authentic one, and use it to calculate the round-trip ToF (hence the distance between both devices). However, that first peak could be due to noise, and similarly many of the following peaks. Those noise peaks may even be artificially added by the adversary to push the receiver into choosing his own peak which is behind the authentic one. Therefore, assuming the first preamble peak is the authentic one is insufficient to mitigate distance-enlargement attacks.
\item Performing these tests on the conventional code will not allow detection -- as attacker know where to annihilate the pulse and where to add. Even on adding energy at $N_p * 2$ pulses will not exceed threshold of test 2 
\item Signals (power) degrade due to channel conditions, which may, \eg make the authentic preamble look like noise.

%--Solutions that won't work
\item Talk about how the receiver cannot rely on the highest preamble peak
\item If the sender and receiver agree on some secret payload, that makes the adversary's objective quite easy.

%--Hints on our solution
\item Emphasise: Our work take more realistic attacker into consideration with the possibility of cancellation, misclassification of attack instance to noise is very low (some value here). It can be deployed alongside secure upper bound estimating techniques, providing security from both attacks in the same platform.
\item Our scheme is based on OOK modulation, the energy of the multiple pulses is aggregated and hypothesis test is applied to detect bit level information.
\end{itemize}

Evaluation:
\begin{itemize}
\item Consider plotting a 3D of zeta on the z-axis, against E and the ratio of D2/D1
\item PDF of attacker's energy?
\item Comment on why we proceed adversary's power same as that of receiver, and what would happen if the adversary uses a different constant power, or varying powers. Future work? Simulations?
\item Setting the number of bogus pulses based on distance/channel condition? if they were really close, may be they don't need to have very long trail of bogus pulses
\item Explain with numbers how much a preamble peak needs to be delayed for how long a distance
\end{itemize}

Proposed Technique:
\begin{itemize}
\item In the implementation, perhaps mention that we have used this paper's technique to find the leading edge. The highest peak can be an attempt of overshadowing attack, looking only at this peak will result into wrong timing estimate. The search-back (SB) and jump-back search-forward (JBSF) algorithms~\cite{Multiple_leading_edge} detect leading edge in the presence of multiple peaks. Our technique leverages the SB algorithm to detect multiple peaks, but the authentic peak is distinguished from others by using payload. The payload is sampled w.r.t to all the peaks selected using distance commitment approach and decision are made using payload samples. 
\end{itemize}

\begin{figure}
	\centering
	\includegraphics[width=1\linewidth]{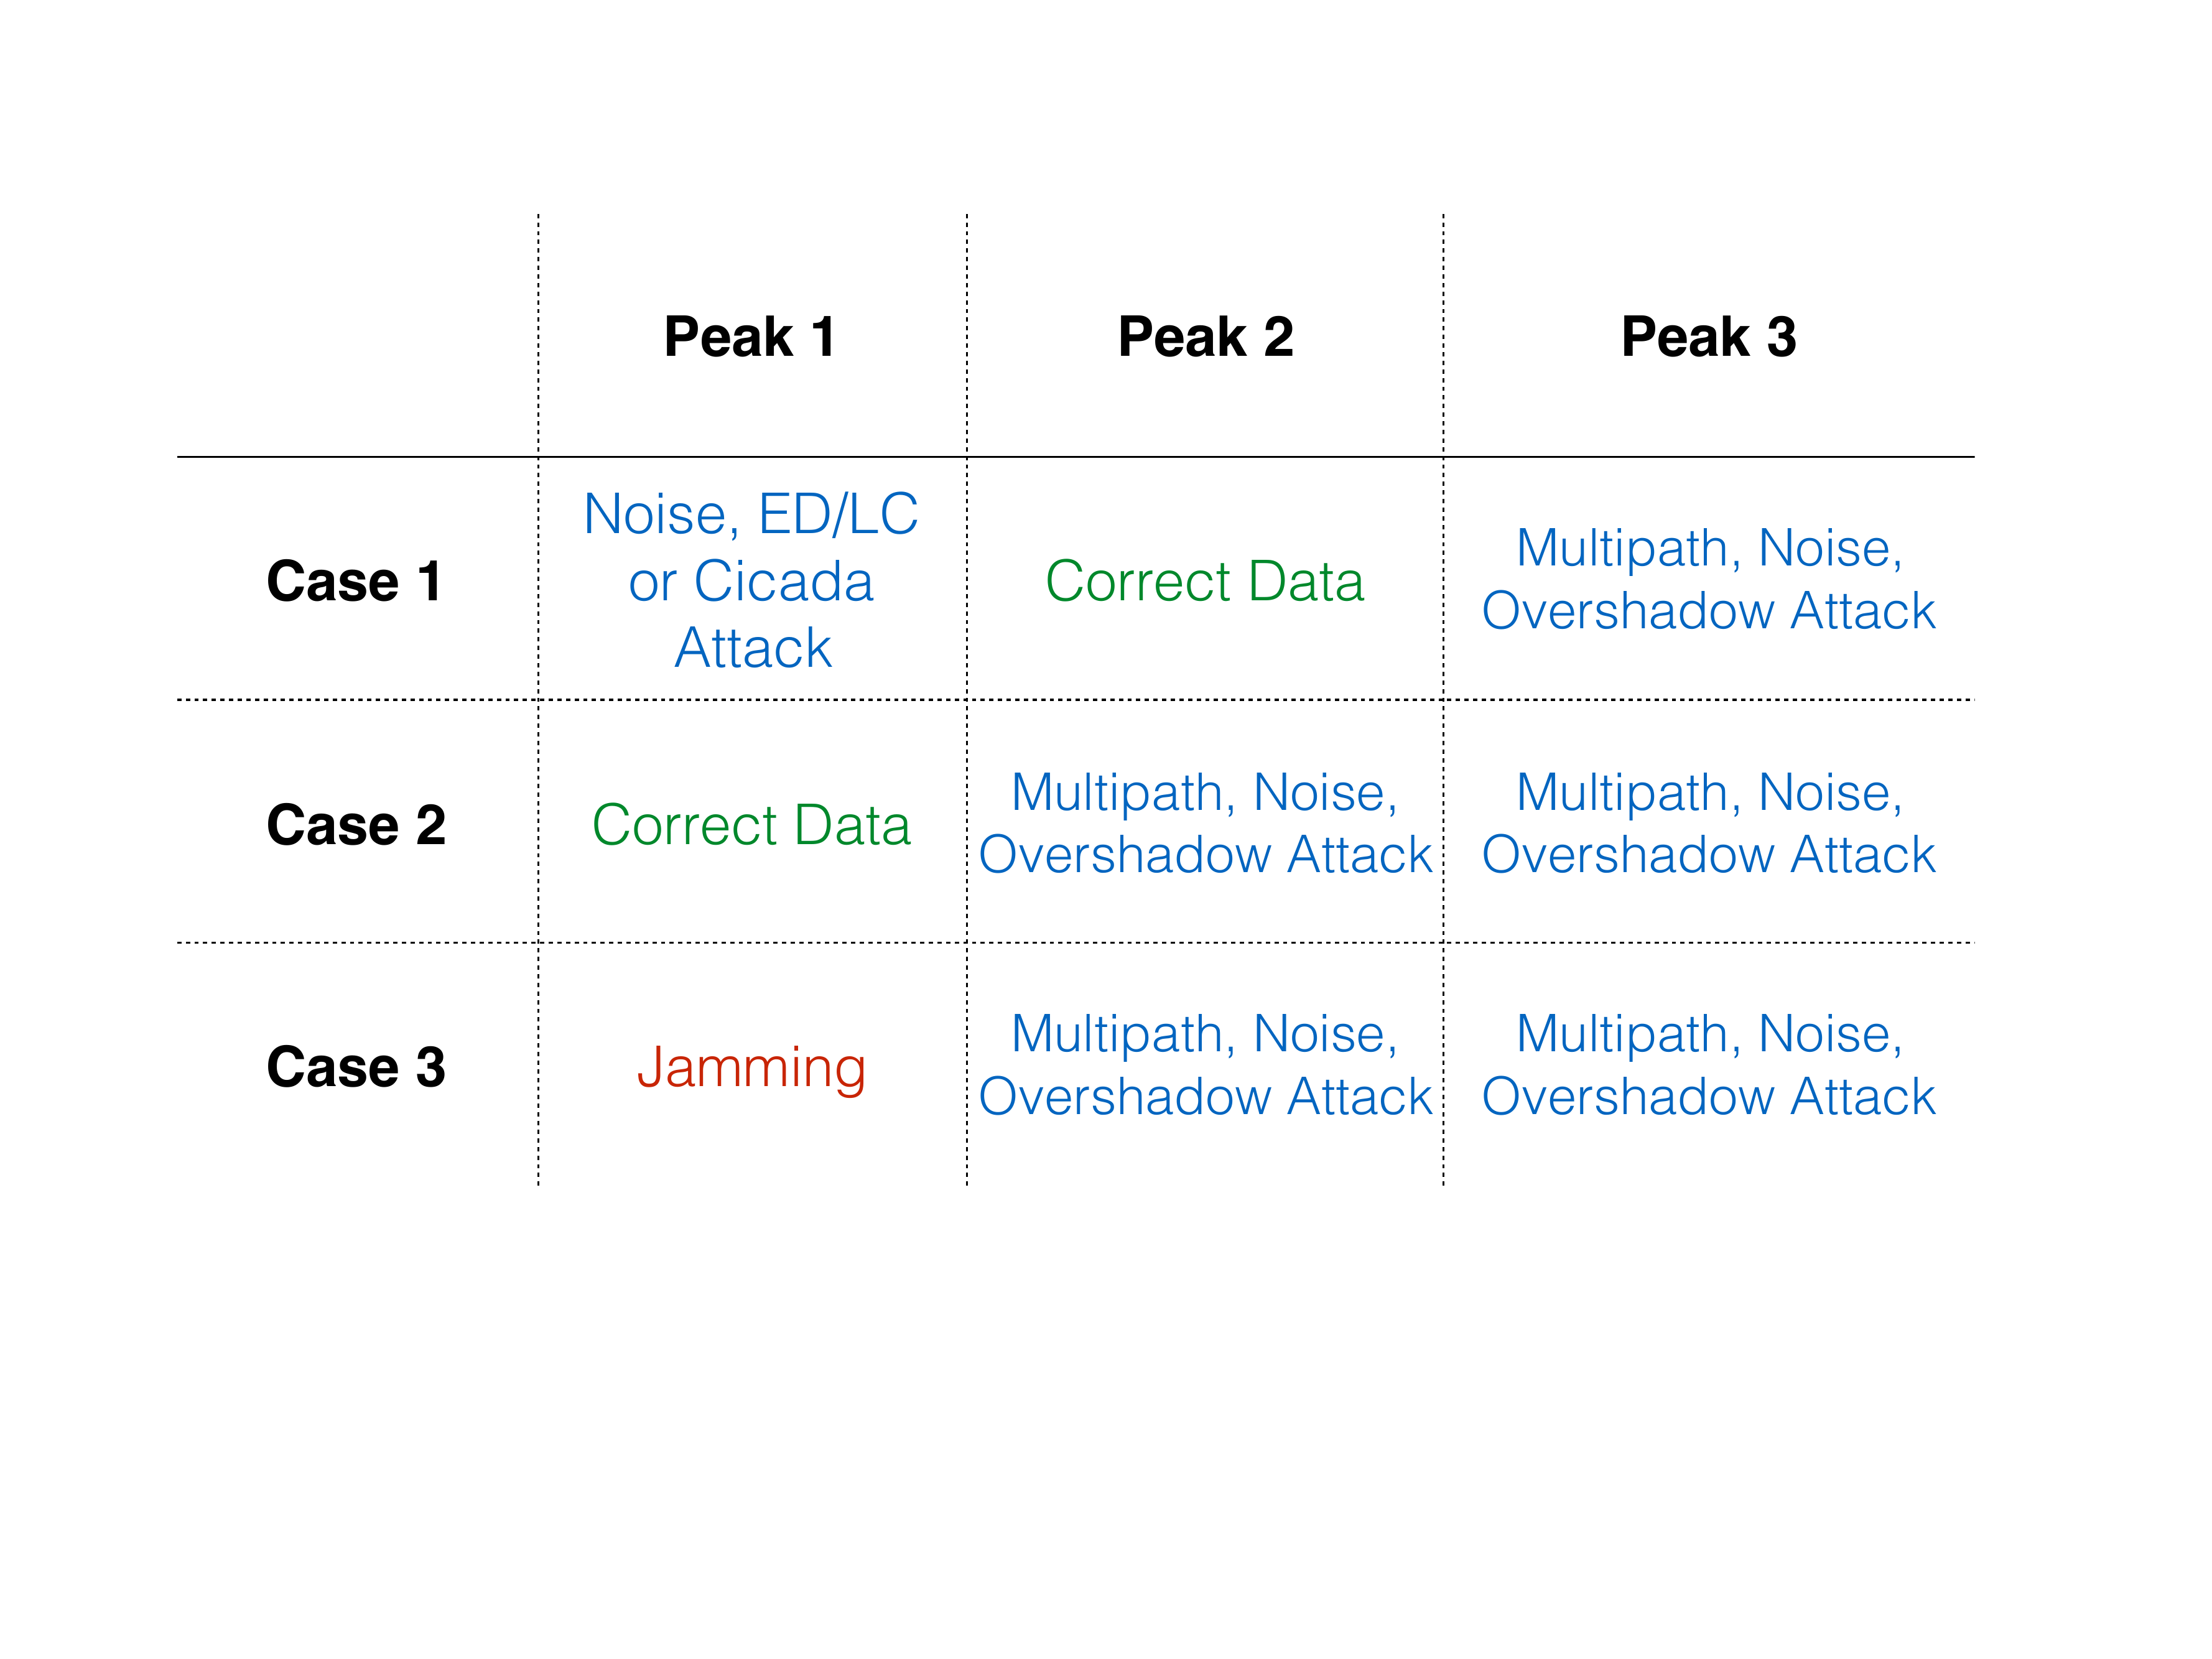}
	\caption{Sampling of payload w.r.t to multiple peaks can result into different payload at receiver. Correct payload can be  preceded by noise or jamming signal. The noise and jamming signal both result in to wrong payload. Jamming signal differ from noise in term of aggregated energy. }
	\label{fig:datablock}
\end{figure}

\subsection{Probability of Not Exceeding Threshold}
\label{sec:probsecondcheck}

We calculate the probability that the overall aggregate energy will not exceed the receiver's threshold (see Section~\ref{sec:settingparam}) after the adversary has added $k$ pulses. We begin by deriving the probability that the overall aggregate has increased by $\delta\ \mu W$. Every adversary-added pulse landing in Bin$_\alpha$ will either cause a reduction or an increase in the overall aggregate.

Assuming $a$ of the $k$ adversary pulses landed in Bin$_\alpha$ and caused an increase in energy, $b$ landed in Bin$_\alpha$ and caused energy reduction, and $c$ landed in Bins 2 and 3 (where $a+b+c=k$), then $\delta$ is such that:
\begin{equation}
\begin{aligned}
\delta	&= a-b+c\\
		&= k-2b \text{\ \ (because }a+c=k-b\text{)}
\end{aligned}
\end{equation}
This leaves a single value for $b$ for the $k$ adversary pulses to result in an aggregate energy increase of exactly $\delta\ \mu W$:
\begin{equation}
\label{eq:bbb}
b=\frac{k-\delta}{2}
\end{equation}
Now for all $x_1$ pulses landing in Bin$_\alpha$ ($x_1=a+b$), we can express the probability that the overall aggregate has increased by $\delta$ as a function of $n$, $\alpha$ and $k$: 
\begin{equation}
p_{n,\alpha,k}(\delta) = \sum_{x_1=(k-\delta)/2}^{k} \left(\frac{\chse{x_1}{(k-\delta)/2}}{2^{x_1}} \cdot \frac{\chse{\alpha}{x_1}\cdot \chse{n-\alpha}{k-x_1}}{\chse{n}{k}}\right)
\end{equation}
This is the probability that $x_1$ adversary pulses fell into Bin$_\alpha$ and the remaining $k-x_1$ fell into Bins 2 and 3, by the probability that $b=(k-\delta)/2$ of those $x_1$ pulses were annihilated. Note that in some cases, the overall aggregate may actually decrease (\eg at $k=1$ adversary pulse, which annihilates a pulse from Bin$_\alpha$). In the extreme case, it can decrease by $k$. Accordingly, because the attack would be detected if the aggregate energy of the received signal exceeds thrshld $=\alpha\gamma$ (or $\gamma$ times the energy originally sent), the probability that the adversary stays within the receiver's threshold is:
\begin{equation}
\label{eq:probatksuccesspart2}
P_{\leq \text{thrshld}}(n, \alpha, k,\gamma) =  \sum_{\delta=-k}^{\alpha(\gamma-1)} p_{n,\alpha,k}(\delta)
\end{equation}

In (\ref{eq:r}), as $R$ increases, the adversary's room of succeeding in distance enlargement increases as well. Figure~\ref{chart:secondcheck} plots the probability of the adversary staying within threshold, $P_{\leq \text{thrshld}}(n, \alpha, k, \gamma)$, for several values of $\gamma$.

\input{sections/charts/second}

The amplified pulses will compensate for the annihilated ones when the receiver choose pulses randomly from the bins for energy comparison, and thus the adversary's chances of success are not expected to substantially improve. See Section~\ref{sec:probsuccess} for calculating its chances of success.

%\begin{equation}
%\begin{aligned}
%(k-2d)\ |\lambda_\text{adversary}| + \alpha\ |\lambda_\text{received}^\text{worst}|	&\leq \gamma\\
%																						&\leq \alpha\ |\lambda_\text{received}^\text{best}|
%\end{aligned}
%\end{equation}

\end{document}
